# Supplementary material for: BEV-IO: Enhancing Bird's-Eye-View 3D Detection with Instance Occupancy
Source: arXiv:2305.16829 source file (2024-01-11)
Supplement: Supplementary file 1 [file X_suppl.tex]

\section{Network Architecture}
Our network architecture is shown in Fig~\ref{fig:network}. The added network parameters of BEV-IO are several 1x1 convolutions. Therefore, the increase in parameter and computation overhead is very small.
\begin{figure}[t]
    \centering
    \includegraphics[width=0.9\textwidth]{sup.pdf}
    \captionsetup{justification=centering}
    \caption{\textbf{Network architecture.}
    }
\label{fig:network}
\end{figure}

\section{Geometry-aware Feature Propagation}
